# Supplementary material for: Generative Organizational Behavior Simulation using Large Language Model based Autonomous Agents: A Holacracy Perspective
Source: arXiv:2408.11826 source file (2024-08-05)
Supplement: Supplementary file 1 [file appendix.tex]

% %Version 3 December 2023
% % See section 11 of the User Manual for version history
% %
% %%%%%%%%%%%%%%%%%%%%%%%%%%%%%%%%%%%%%%%%%%%%%%%%%%%%%%%%%%%%%%%%%%%%%%
% %%                                                                 %%
% %% Please do not use \input{...} to include other tex files.       %%
% %% Submit your LaTeX manuscript as one .tex document.              %%
% %%                                                                 %%
% %% All additional figures and files should be attached             %%
% %% separately and not embedded in the \TeX\ document itself.       %%
% %%                                                                 %%
% %%%%%%%%%%%%%%%%%%%%%%%%%%%%%%%%%%%%%%%%%%%%%%%%%%%%%%%%%%%%%%%%%%%%%

% %%\documentclass[referee,sn-basic]{sn-jnl}% referee option is meant for double line spacing

% %%=======================================================%%
% %% to print line numbers in the margin use lineno option %%
% %%=======================================================%%

% %%\documentclass[lineno,sn-basic]{sn-jnl}% Basic Springer Nature Reference Style/Chemistry Reference Style

% %%======================================================%%
% %% to compile with pdflatex/xelatex use pdflatex option %%
% %%======================================================%%

% %%\documentclass[pdflatex,sn-basic]{sn-jnl}% Basic Springer Nature Reference Style/Chemistry Reference Style


% %%Note: the following reference styles support Namedate and Numbered referencing. By default the style follows the most common style. To switch between the options you can add or remove Numbered in the optional parenthesis. 
% %%The option is available for: sn-basic.bst, sn-vancouver.bst, sn-chicago.bst%  
 
% %%\documentclass[pdflatex,sn-nature]{sn-jnl}% Style for submissions to Nature Portfolio journals
% %%\documentclass[pdflatex,sn-basic]{sn-jnl}% Basic Springer Nature Reference Style/Chemistry Reference Style
% \documentclass[pdflatex,sn-mathphys-num]{sn-jnl}% Math and Physical Sciences Numbered Reference Style 
% %%\documentclass[pdflatex,sn-mathphys-ay]{sn-jnl}% Math and Physical Sciences Author Year Reference Style
% %%\documentclass[pdflatex,sn-aps]{sn-jnl}% American Physical Society (APS) Reference Style
% %%\documentclass[pdflatex,sn-vancouver,Numbered]{sn-jnl}% Vancouver Reference Style
% %%\documentclass[pdflatex,sn-apa]{sn-jnl}% APA Reference Style 
% %%\documentclass[pdflatex,sn-chicago]{sn-jnl}% Chicago-based Humanities Reference Style

% %%%% Standard Packages
% %%<additional latex packages if required can be included here>

% \usepackage{graphicx}%
% \usepackage{multirow}%
% \usepackage{amsmath,amssymb,amsfonts}%
% \usepackage{amsthm}%
% \usepackage{mathrsfs}%
% \usepackage[title]{appendix}%
% \usepackage{xcolor}%
% \usepackage{textcomp}%
% \usepackage{manyfoot}%
% \usepackage{booktabs}%
% \usepackage{algorithm}%
% \usepackage{algorithmicx}%
% \usepackage{algpseudocode}%
% \usepackage{listings}%
% %%%%

% %%%%%=============================================================================%%%%
% %%%%  Remarks: This template is provided to aid authors with the preparation
% %%%%  of original research articles intended for submission to journals published 
% %%%%  by Springer Nature. The guidance has been prepared in partnership with 
% %%%%  production teams to conform to Springer Nature technical requirements. 
% %%%%  Editorial and presentation requirements differ among journal portfolios and 
% %%%%  research disciplines. You may find sections in this template are irrelevant 
% %%%%  to your work and are empowered to omit any such section if allowed by the 
% %%%%  journal you intend to submit to. The submission guidelines and policies 
% %%%%  of the journal take precedence. A detailed User Manual is available in the 
% %%%%  template package for technical guidance.
% %%%%%=============================================================================%%%%

% %% as per the requirement new theorem styles can be included as shown below
% \theoremstyle{thmstyleone}%
% \newtheorem{theorem}{Theorem}%  meant for continuous numbers
% %%\newtheorem{theorem}{Theorem}[section]% meant for sectionwise numbers
% %% optional argument [theorem] produces theorem numbering sequence instead of independent numbers for Proposition
% \newtheorem{proposition}[theorem]{Proposition}% 
% %%\newtheorem{proposition}{Proposition}% to get separate numbers for theorem and proposition etc.

% \theoremstyle{thmstyletwo}%
% \newtheorem{example}{Example}%
% \newtheorem{remark}{Remark}%

% \theoremstyle{thmstylethree}%
% \newtheorem{definition}{Definition}%

% \raggedbottom
% %%\unnumbered% uncomment this for unnumbered level heads

% \begin{document}

% \title[Agent]{Appendices for Building An Automated Organizational Governance By Large Language Model-Based Agent}

% %%=============================================================%%
% %% GivenName	-> \fnm{Joergen W.}
% %% Particle	-> \spfx{van der} -> surname prefix
% %% FamilyName	-> \sur{Ploeg}
% %% Suffix	-> \sfx{IV}
% %% \author*[1,2]{\fnm{Joergen W.} \spfx{van der} \sur{Ploeg} 
% %%  \sfx{IV}}\email{iauthor@gmail.com}
% %%=============================================================%%


% %%==================================%%
% %% Sample for unstructured abstract %%
% %%==================================%%


% %%\pacs[JEL Classification]{D8, H51}

% %%\pacs[MSC Classification]{35A01, 65L10, 65L12, 65L20, 65L70}

% \maketitle



% \begin{appendices}

% \section{Section title of first appendix}\label{secA1}

% An appendix contains supplementary information that is not an essential part of the text itself but which may be helpful in providing a more comprehensive understanding of the research problem or it is information that is too cumbersome to be included in the body of the paper.



% \end{appendices}


% \bibliography{reference}


% \end{document}
